# Supplementary material for: Heterogeneous Graph Contrastive Learning for Recommendation
Source: arXiv:2303.00995 source file (2023-03-02)
Supplement: Supplementary file 1 [file appendix.tex]

\section{Supplemental Material}
\label{sec:appendix}
